# Supplementary material for: Optical spatial dispersion via Wannier interpolation
Source: arXiv:2504.09742 ancillary file (2025-04-17)
Supplement: Supplementary file 1 [file Supplementary_Material.pdf]

# Supplementary Material for "Optical spatial dispersion via Wannier interpolation"

Andrea Urru,[1,*] Ivo Souza,[2,3,*] Óscar Pozo Ocaña,[2] Stepan S. Tsirkin,[2,3,4] and David Vanderbilt[1]

[1] *Department of Physics & Astronomy, Rutgers University, Piscataway, New Jersey 08854, USA*
[2] *Centro de Física de Materiales, Universidad del País Vasco, 20018 San Sebastián, Spain*
[3] *Ikerbasque Foundation, 48013 Bilbao, Spain*
[4] *Chair of Computational Condensed Matter Physics, Institute of Physics, École Polytechnique Fédérale de Lausanne (EPFL), CH-1015 Lausanne, Switzerland*

## I. WORKFLOW

We present in Fig. S1 a more detailed version of the workflow chart shown in Fig. 3 of the main text. We describe every step necessary to compute by Wannier interpolation the building blocks of the spatially dispersive optical conductivity $\sigma_{\alpha\beta\gamma}(\omega)$. For each step, we provide a reference to the relevant equations in the main text.

## II. CONSTRUCTION OF THE WANNIER FUNCTIONS

Here we report the relevant computational details relative to the wannierization of the *ab initio* electronic structure of the four materials studied: wurtzite GaN, trigonal Te, trigonal Se, and $\alpha$-quartz. In Table SI we list for each material the trial orbitals used to build the Wannier basis, and the range of the frozen energy window used in the disentanglement step. In Fig. S2 we show the Wannier-interpolated electronic bands compared with the *ab initio* band structure. For clarity, we highlight the frozen windows in the band structure plots as well. Note that we do not provide a comparative bandstructure plot for Te; for this material we used a hybrid functional, which does not allow for a straightforward calculation of the energy bands along an arbitrary path by means of a standard non-self-consistent calculation.

## III. AUGMENTED WANNIER BASIS FOR TRIGONAL SELENIUM

As discussed in the main text, in order to assess the band-truncation error in the calculation of the rotatory power of trigonal Se, more conduction bands need to be wannierized. Including additional atom-centered trial orbitals such as $4d$ or $5s$ does not yield an accurate band interpolation, suggesting that the conduction states above those of $4p$ character are interstitial states. To get a reasonably accurate Wannier description of such states, we adopt the SCDM method [1, 2]. Since $4s$ and $4p$ states already provide an accurate description of the highest nine valence bands and lowest three conduction bands (Fig. S2(b)), we only use the SCDM method to wannierize conduction bands above the three lowest ones. As interstitial sites are usually located at general Wyckoff positions, their multiplicity is equal to the number of symmetry operations of the full crystal point group. For Se, this means that interstitial states are grouped in sets of six elements. In the following, we discuss the results obtained with 12 interstitial Wannier functions.

In Fig. S3(a) we show the interpolated bands obtained with the SCDM method as outlined above. The positions of the 12 interstitial Wannier centers is shown in Fig. S3(b). These are clearly grouped in two families: an inner one (centers 1-6 in the figure) close to Se atoms, and an outer one (centers 7-12) close to the boundary of the Wigner-Seitz cell, identified by the black hexagon. Within each family, the centers should be related to each other by symmetry; however, symmetry is inherently broken by the SCDM algorithm. Thus, we symmetrize the set of interstitial Wannier centers by picking one representative from each family and applying to it the symmetry operations of space group $P3_121$ to generate the other five centers. The resulting set of centers is shown in Fig. S4(a). Finally, we perform a Wannier interpolation to interpolate both the $s$-$p$ manifold and the interstitial states. To this end, we adopt a set of trial orbital comprising $s$ and $p$ orbitals centered on Se atoms, and 12 $s$ orbitals located at the Wannier centers symmetrized as explained above. The resulting interpolated bands are shown in Fig. S4(b) together with *ab initio* bands.

---

* These authors contributed equally to the manuscript.

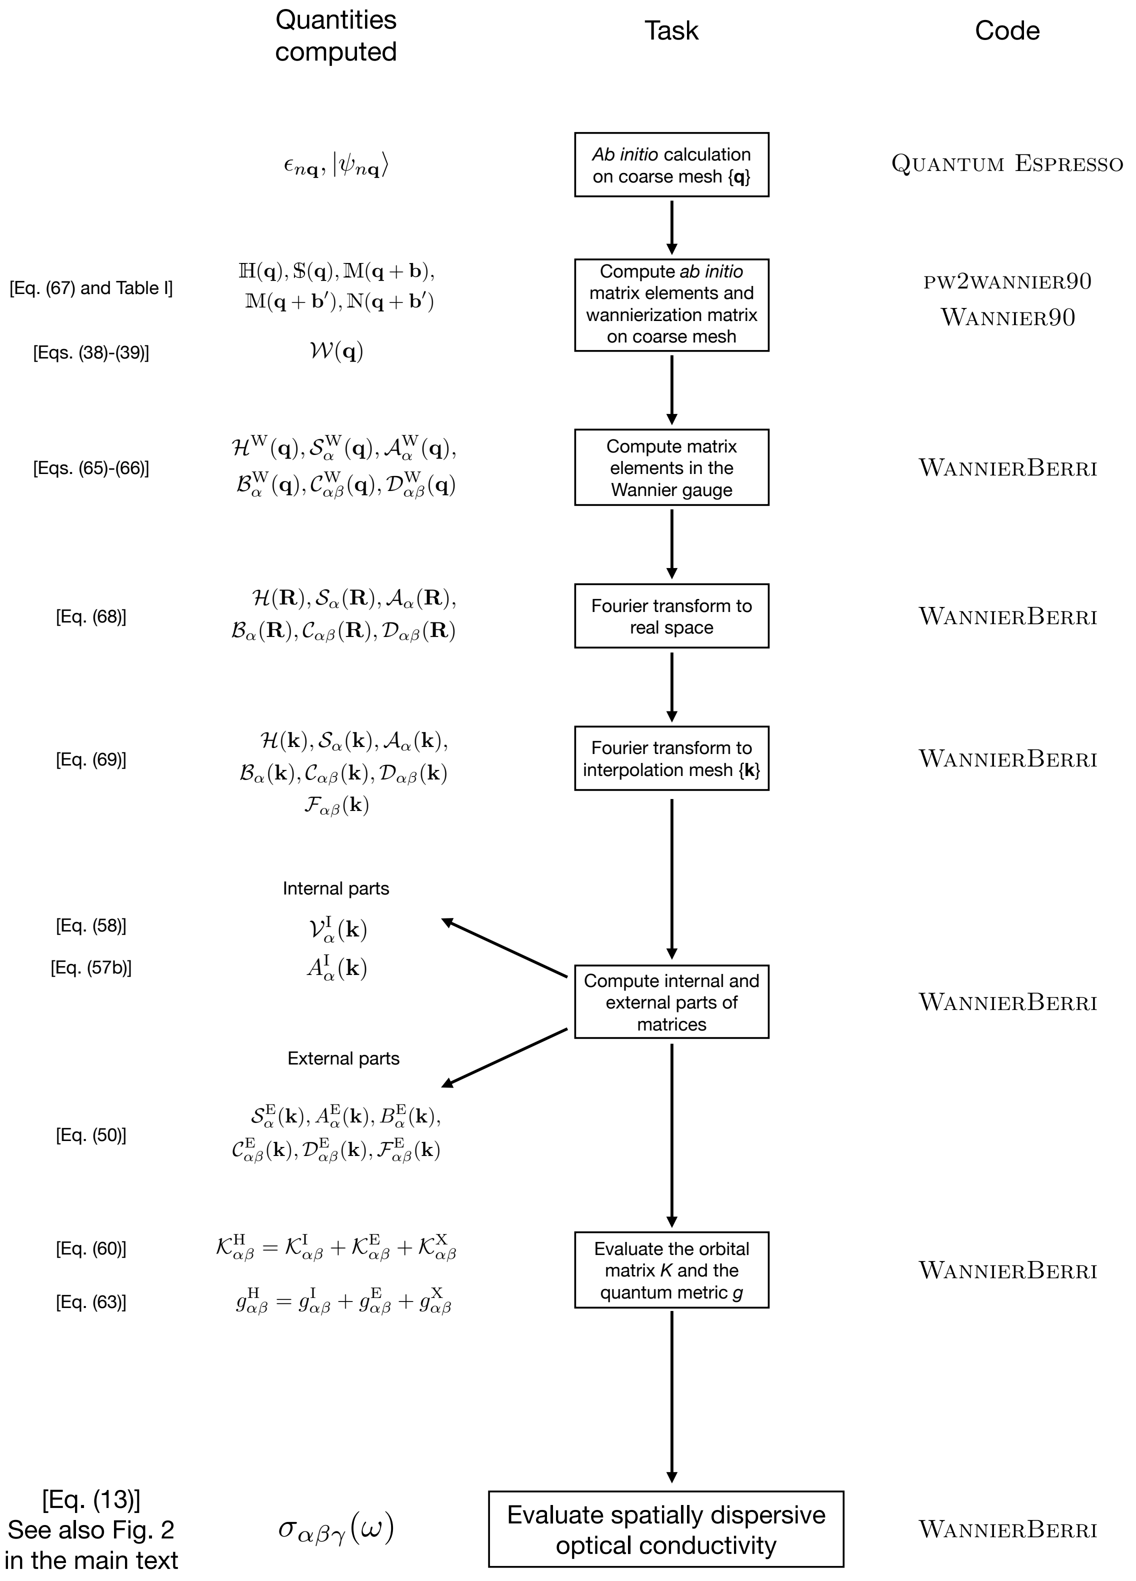


FIG. S1. Workflow to compute the spatially dispersive optical conductivity using Wannier interpolation.

TABLE SI. Trial functions and energy range (relative to the Fermi energy) of the frozen window used for constructing the Wannier functions.

| Compound | Trial functions | Frozen window energy range |
|---|---|---|
| GaN | Ga: $s$, $p$; N: $p$ | from $-10$ eV to 11 eV |
| Te | Te: $s$, $p$ | from $-20$ eV to 3 eV |
| Se | Se: $s$, $p$ | from $-7.5$ eV to 3 eV |
| $\alpha$-$SiO_2$ | Si: $s$, $p$; O: $p$ | from $-11$ eV to 12 eV |

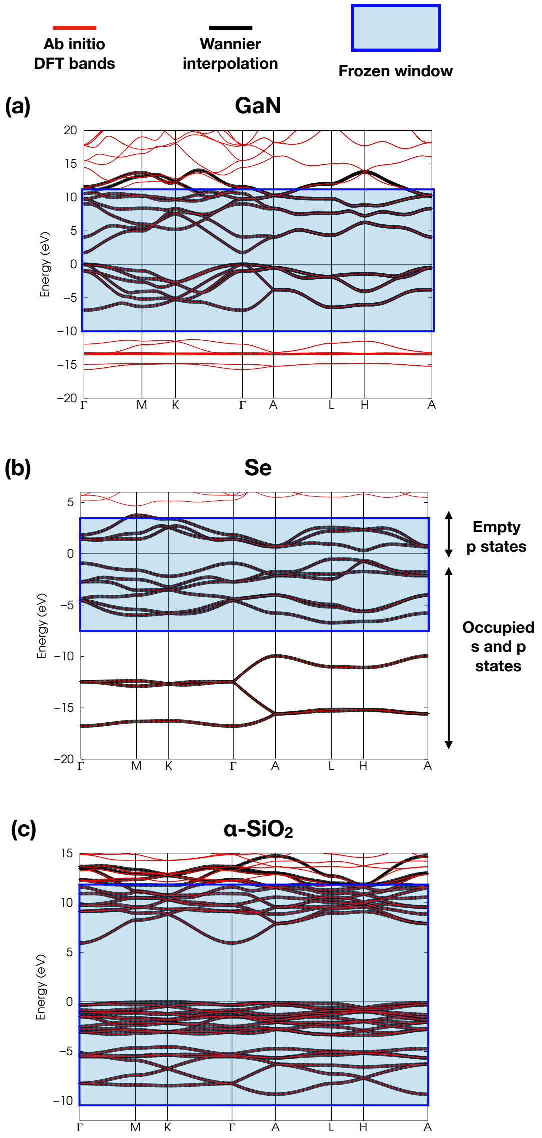


FIG. S2. Wannier-interpolated electronic bands compared with *ab initio* band structures for GaN, Se, and $\alpha$-$SiO_2$. The shaded blue rectangle identifies the frozen energy window used in the disentanglement step of the Wannier construction.

[1] A. Damle, L. Lin, and L. Ying, Compressed representation of Kohn–Sham orbitals via selected columns of the density matrix, J. Chem. Theory Comput. **11**, 1463 (2015).

[2] A. Damle and L. Lin, Disentanglement via entanglement: A unified method for Wannier localization, Multiscale Model. Simul. **16**, 1392 (2018).

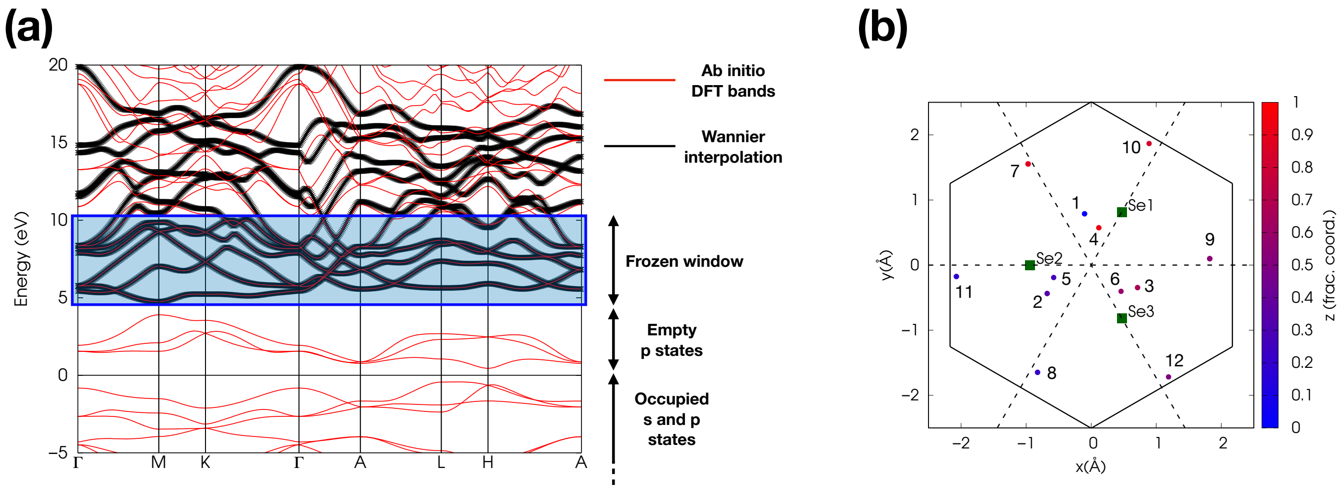


FIG. S3. (a) Wannier interpolation performed with the SCDM method on the empty states located above the s-p manifold. (b) Wannier centers as obtained from the SCDM method. The black hexagon represents the Wigner-Seitz cell, the green squares indicate the position of Se atoms projected onto the $xy$ plane, and the circles identify the position of Wannier centers.

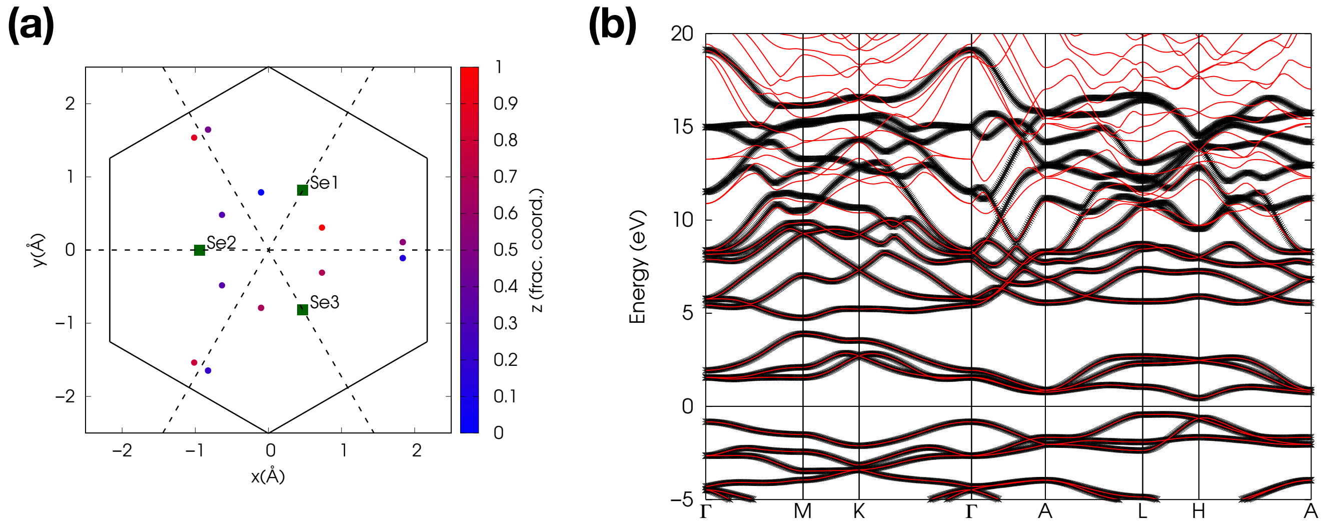


FIG. S4. (a) Positions of the starting interstitial trial functions. (b) Wannier-interpolated electronic structure obtained starting from a set of trial functions containing $s$ and $p$ orbitals on Se sites, and $s$ orbitals on the interstitial sites reported in panel (a).
